# Supplementary material for: Don't Throw it Away! The Utility of Unlabeled Data in Fair Decision Making
Source: arXiv:2205.04790 source file (2022-07-04)
Supplement: Supplementary file 2 [file scb.tex]

\tikz{
% nodes
 \node[obs](s) {S};
 \node[obs,right=1cm of s] (l) {LSAT};
 \node[obs, above=of l,  yshift=-0.5cm] (g) {GPA}; 
 \node[obs, below=of l, yshift=0.5cm] (f) {FYA}; 
 \node[latent,right=1cm of l] (k) {K};
% edges
 \edge {s} {g, l, f}
 \edge {k} {g, l, f}
 }
